# Supplementary material for: ARTrackV2: Prompting Autoregressive Tracker Where to Look and How to Describe
Source: arXiv:2312.17133 source file (2024-02-13)
Supplement: Supplementary file 1 [file _supplementary.tex]

% \input{_constants}
% \review % \review OR \cameraready

% \documentclass[10pt,twocolumn,letterpaper]{article}
% \input{cvpr_header}
% \myexternaldocument{_main}
% \begin{document}
% %% TITLE
% \title{\paperTitle \\ Supplemental Material}
% \author{\authorBlock}
% \maketitle
% %%

% %\twocolumn[{
% %}]

% \input{12_appendix}

% {\small
% \bibliographystyle{ieee_fullname}
% \bibliography{11_references}
% }

% \end{document}
